# Supplementary material for: Thermal transport of glasses via machine learning driven simulations
Source: arXiv:2402.06479 ancillary file (2024-02-09)
Supplement: Supplementary file 1 [file supplementary.pdf]

# Supplementary Material to
# *Thermal transport of glasses via machine learning driven simulations*

Paolo Pegolo [1] and Federico Grasselli [2]

[1] *SISSA—Scuola Internazionale Superiore di Studi Avanzati, Trieste*
[2] *COSMO—Laboratory of Computational Science and Modeling, IMX, École Polytechnique Fédérale de Lausanne, 1015 Lausanne, Switzerland*

(Dated: February 9, 2024)

## I. VITREOUS SILICA DATASET

The silica Tersoff dataset [1] is generated starting from 100 independently quenched glassy samples, equilibrated at 10 different temperatures ranging from 300 K to 7000 K. The melt-quench-anneal procedure consists of melting a crystalline (quartz) sample at 7000 K, then quenching it to 500 ps at a quenching rate of $2.6 \cdot 10^{12}\,\mathrm{K\,s^{-1}}$, followed by 125 ps of tempering at 500 K. The 100 independent samples are used as initial configurations to start zero-pressure simulations at ten different temperatures ranging from 300 K to 7000 K. From each of these simulations, 500 uncorrelated configurations are drawn once every 10 ps. The dataset thus comprises around 50,000 glassy and molten configurations.

The validation set is generated analogously and comprises 2,500 configurations.

### A. DP training

The size of the embedding net is (25, 50, 100), and the size of the fitting net is (240, 240, 240). The cutoff radius is set to 3 Å, and the smoothing parameter `rcut_smth` at 0.5 Å. The stochastic gradient descent scheme Adam [2] is employed for $5 \cdot 10^7$ steps to train the DP models. The hyperparameters `start_pref_e`, `start_pref_f`, `start_pref_v`, `limit_pref_e`, `limit_pref_f`, and `limit_pref_v`, which govern the weights of energy, force, and virial losses in the total loss function, are set to 0.02, 1000, 0.01, 1.0, 1.0, and 1.0, respectively. The initial learning rate is 0.001, and it exponentially decays to $3.5 \cdot 10^{-8}$ by the end of the training.

### B. NEP training

Both angular and radial cutoffs are set to 3 Å. Radial and angular descriptors feature 4 components [3] and are built out of 12 functions. The parameters governing angular expansion order [3], `l_max`, are set to (4, 2, 0). The number of neurons in the hidden layer is 30. The weights of the loss term associated with energy, forces, and virial are set to 1.0, 1.0, and 0.1, respectively. The genetic optimization is carried out on batches of 5000 configurations. The population size and number of generations of the SNES algorithm [4] are set to 50 and $2 \cdot 10^6$, respectively.

## II. LITHIUM-INTERCALATED AMORPHOUS SILICON

### A. NEP training

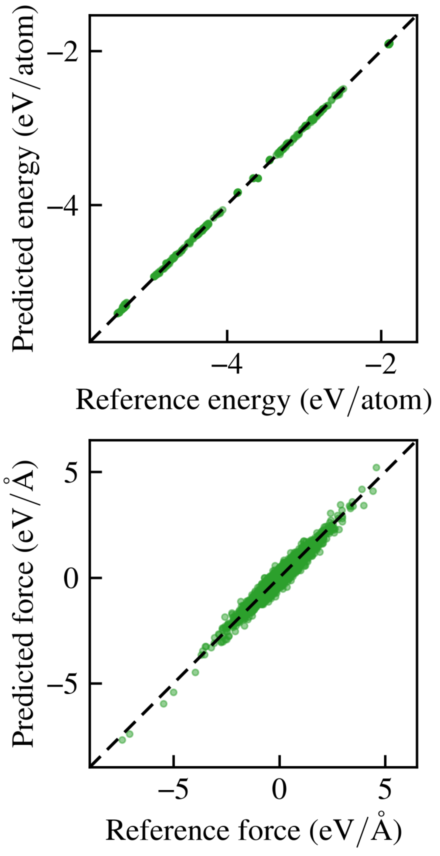


FIG. 1. Parity plots for the NEP trained on the $Li_xSi_{1-x}$ dataset.

We trained a NEP on the dataset taken from Ref. 5. Radial and angular cutoffs are set to 6 and 4 Å, respectively. Both Radial and angular descriptors feature 10 components [3] and are built out of 12 functions. The parameters governing angular expansion order [3], `l_max`,

are set to (4, 2, 0). The number of neurons in the hidden layer is 30. The weights of the loss term associated with energy, forces, and virial are set to 1.0, 1.0, and 0.0, respectively. The genetic optimization is carried out on batches of 500 configurations. The population size and number of generations of the SNES algorithm [4] are set to 50 and $4 \cdot 10^5$, respectively.

The parity plots for this NEP on a validation set are shown in Fig. 1. The RMSEs on energy and forces are $13\,\mathrm{meV\,atom^{-1}}$ and $82\,\mathrm{meV\,Å^{-1}}$, respectively. The former agrees with the one of the DP of Ref. 5, while the latter outperforms it by a factor of two.

### B. Equilibrium molecular dynamics simulations

Equilibrium molecular dynamics simulations to compute the thermal conductivity of $Li_xSi_{1-x}$ are carried out with GPUMD [3]. Samples with varying Li concentration are prepared through a melt-quench-anneal procedure [5] consisting of a melting phase starting at 2500 K and ending at 1800 K for 200 ps, followed by three quenching phases: *i)* from 1500 to 1250 K at a rate of $10^{13}\,\mathrm{K\,s^{-1}}$; *ii)* from 1250 to 1050 K at a rate of $10^{11}\,\mathrm{K\,s^{-1}}$; *iii)* from 1050 to 500 K at a rate of $10^{13}\,\mathrm{K\,s^{-1}}$. The atomic positions are further minimized to achieve mechanical equilibrium up to a force tolerance of $10^{-6}\,\mathrm{eV\,Å^{-1}}$.

The amorphous configurations so obtained are used as initial states for canonical [6] EMD simulations. After 300 ps of canonical equilibration at 300 K, the energy and mass fluxes are sampled for 3 ns and subsequently analyzed through the cepstral method [7] with the SporTran code [8] to obtain the thermal conductivity. The fluxes' resampling frequency [7, 8] is set to 5 THz.

[1] S. Munetoh, T. Motooka, K. Moriguchi, and A. Shintani, Interatomic potential for si–o systems using tersoff parameterization, Computational Materials Science **39**, 334 (2007).

[2] D. P. Kingma and J. Ba, Adam: A method for stochastic optimization (2017), arXiv:1412.6980 [cs.LG].

[3] Z. Fan, Y. Wang, P. Ying, K. Song, J. Wang, Y. Wang, Z. Zeng, K. Xu, E. Lindgren, J. M. Rahm, *et al.*, GPUMD: A package for constructing accurate machine-learned potentials and performing highly efficient atomistic simulations, J. Chem. Phys. **157**, 114801 (2022).

[4] T. Schaul, T. Glasmachers, and J. Schmidhuber, High dimensions and heavy tails for natural evolution strategies, in *Proceedings of the 13th Annual Conference on Genetic and Evolutionary Computation*, GECCO '11 (Association for Computing Machinery, New York, NY, USA, 2011) p. 845–852.

[5] F. Fu, X. Wang, L. Zhang, Y. Yang, J. Chen, B. Xu, C. Ouyang, S. Xu, F.-Z. Dai, and W. E, Unraveling the atomic-scale mechanism of phase transformations and structural evolutions during (de)lithiation in si anodes, Advanced Functional Materials **33**, 2303936 (2023).

[6] G. Bussi, D. Donadio, and M. Parrinello, Canonical sampling through velocity rescaling, J. Chem. Phys. **126**, 014101 (2007).

[7] L. Ercole, A. Marcolongo, and S. Baroni, Accurate thermal conductivities from optimally short molecular dynamics simulations, Sci. Rep. **7**, 1 (2017).

[8] L. Ercole, R. Bertossa, S. Bisacchi, and S. Baroni, Sportran: A code to estimate transport coefficients from the cepstral analysis of (multivariate) current time series, Computer Physics Communications **280**, 108470 (2022).
